# Supplementary material for: Carrier-envelope phase effects in Laser Wakefield Acceleration with near-single-cycle pulses
Source: arXiv:2006.10566 ancillary file (2020-10-14)
Supplement: Supplementary file 1 [file SupplementaryInformation.pdf]

# Identifying observable carrier-envelope phase effects in Laser Wakefield Acceleration with near-single-cycle pulses
# - Supplementary Information -

Julius Huijts,[1] Igor A. Andriyash,[1] Lucas Rovige,[1] Aline Vernier,[1] and Jérôme Faure[1]

[1] *Laboratoire d'Optique Appliquée, CNRS, Ecole Polytechnique, ENSTA Paris, Institut Polytechnique de Paris, 181 Chemin de la Hunière et des Joncherettes, 91120 Palaiseau, France*

(Dated: September 8, 2020)

## I. INTENSITY SCALING BEAM PARAMETERS

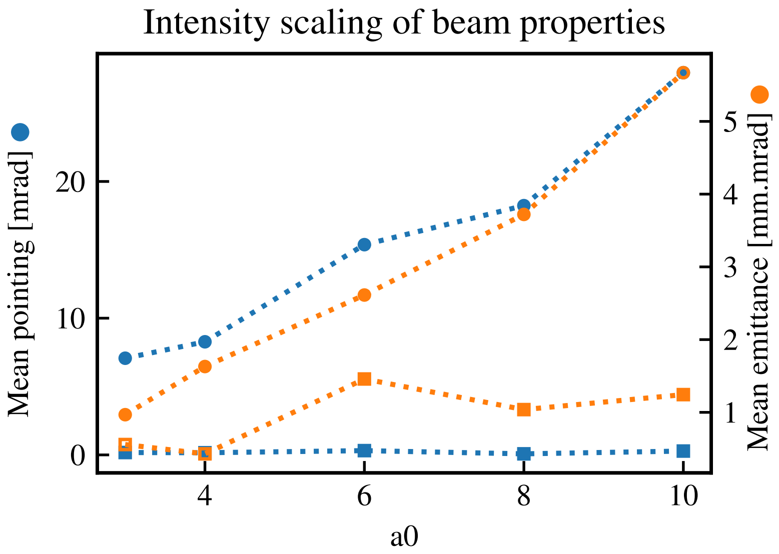


FIG. 1: Behavior of electron beam properties with increasing intensity. The dots indicate the mean absolute pointing (blue) and transverse normalized emittance (orange) in the plane of polarization. Both the pointing and the emittance show a clear increase with laser intensity. The squares correspond to pointing and emittance in the perpendicular plane (the mean absolute pointing in this plane is zero as expected). The dotted lines are guides to the eye.

## II. ELECTRON BEAM AND LASER PULSE EVOLUTION FOR $a_0 = 4$ (SELF-INJECTION)

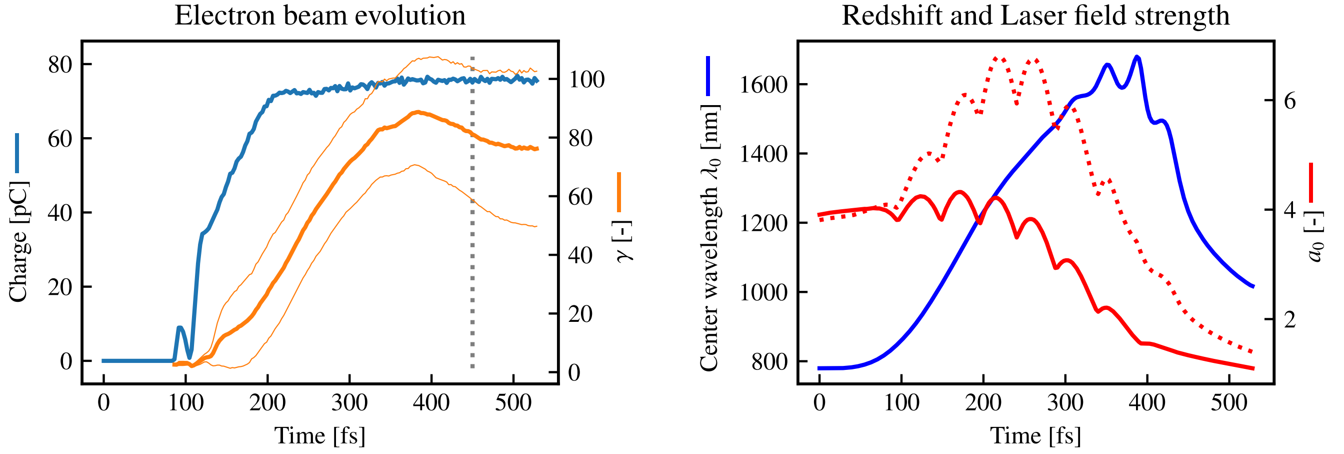


(a) Total beam charge (blue) as a function of time, showing the the injection takes place from 140 fs to 200 fs, as well as the evolution of the mean energy ($\gamma$, orange). The thin orange lines indicate the rms energy spread.

(b) The center wavelength of the pulse (blue), showing a strong redshift of up to factor 2. In red, the normalized peak laser field strength $a_0$, normalized to the vacuum wavelength (solid) and to the redshifted wavelength (dotted).

FIG. 2

## III. ELECTRON BEAM AND LASER PULSE EVOLUTION FOR $a_0 = 3$ (DG-INJECTION)

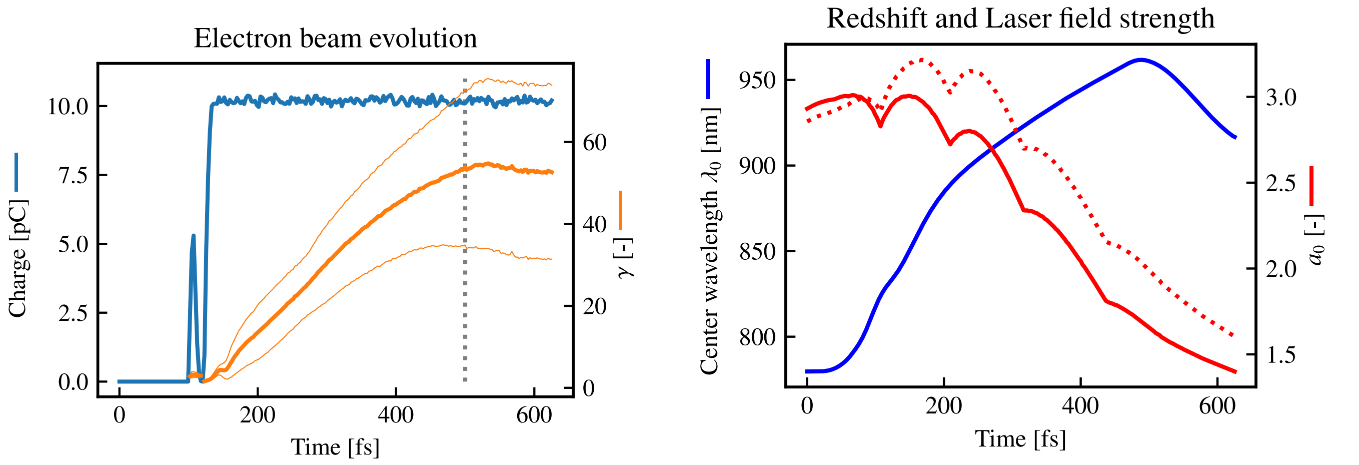


(a) Total beam charge (blue) as a function of time, showing that the injection is instantaneous at 125 fs, as well as the evolution of the mean energy ($\gamma$, orange). The thin orange lines indicate the rms energy spread.

(b) The center wavelength of the pulse (blue) is redshifted by about 20 % over the course of the simulation. In red, the normalized peak laser field strength $a_0$, normalized to the vacuum wavelength (solid) and to the redshifted wavelength (dotted)

FIG. 3

## IV. CIRCULAR POLARIZATION

The case of circular polarization was investigated by repeating the self injection simulation ($a_0 = 4, \phi_i = 0$) with an initial laser pulse given by:

$$\vec{\Psi}_{circ} = 1/\sqrt{2}\left[\Psi_0(\phi_i = 0)\hat{x} + \Psi_0(\phi_i = \pi/2)\hat{y}\right], \tag{1}$$

where $\Psi_0$ designates the (linearly polarized) pulse used in the simulations in the main text. Hence, the circularly polarized pulse is a superposition of two linearly polarized pulses, one in the $\hat{x}$- and one in the $\hat{y}$-direction, where the second pulse is delayed by $\pi/2$. The plasma response can also be seen as a superposition of the linear plasma response in the x- and y-plane, with a $\pi/2$ phase difference (figure 4a). This gives thus a rotary motion with an amplitude that increases up to about 280 fs and then decreases, as is clear from figure 4b. The evolution of the pointing of the electron beam in $x$ (figure5a) is similar to the linearly polarized case, whereas the evolution of the pointing in $y$ is similar to the linearly polarized case for $\phi_i = \pi/2$. Their superposition yields the motion depicted in figure 5b. This motion is the result of the interplay between the bubble oscillation and the betatron oscillation. As such, the three-blade propeller shape apparent in the beam motion especially between 250 and 400 fs has a straightforward explanation: mathematically such a shape is obtained by the superposition of two counterrotating motions, with frequencies $\omega_1$ and $\omega_2 = -2\omega_1$. Indeed, between 250 and 400 fs the betatron period ($T_\beta = 2\pi\sqrt{(}2\gamma)/\omega_p$) increases from 170 to 230 , while $T_{2\pi} = 108$ fs.The total charge and energy of the electron beam (figure 6) for circular polarization is similar to the case of linear polarization (see figure 3a).

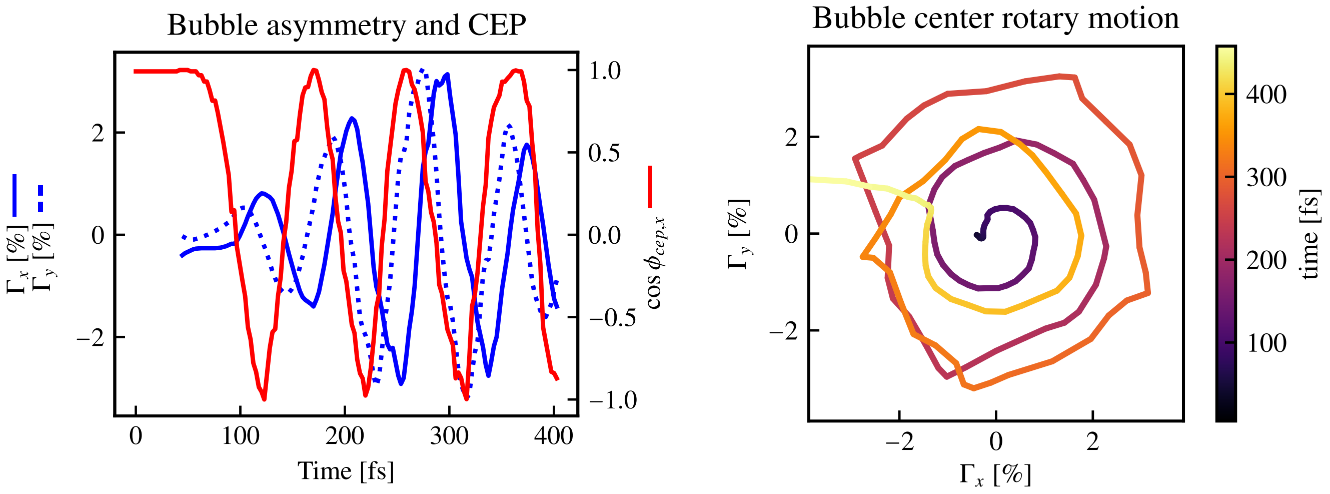


(a) Asymmetry of the bubble for the case of circular polarization, in the x- and y-plane (solid and dotted blue resp.), and the carrier-envelope phase of the driving laser pulse in x (red).

(b) Asymmetry of the bubble plotted in the xy-plane, clearly showing the circular motion of the bubble behind the laser pulse.

FIG. 4

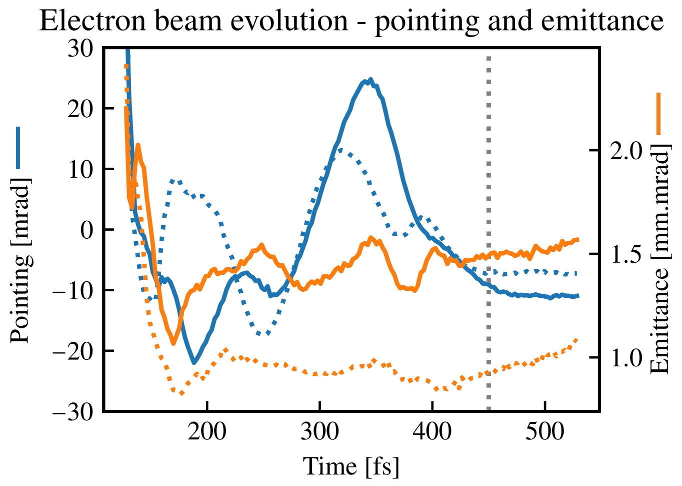


(a) Circular polarization: evolution of the electron beam pointing (blue) and emittance (orange) in $x$ (solid) and $y$ (dotted).

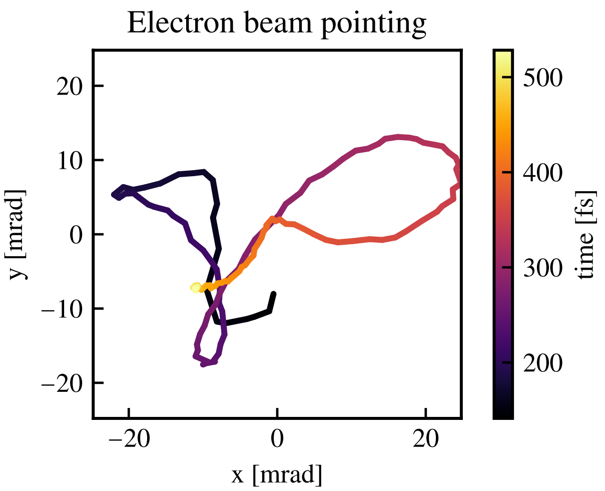


(b) Circular polarization: the electron beam pointing plotted in the xy-plane.

FIG. 5

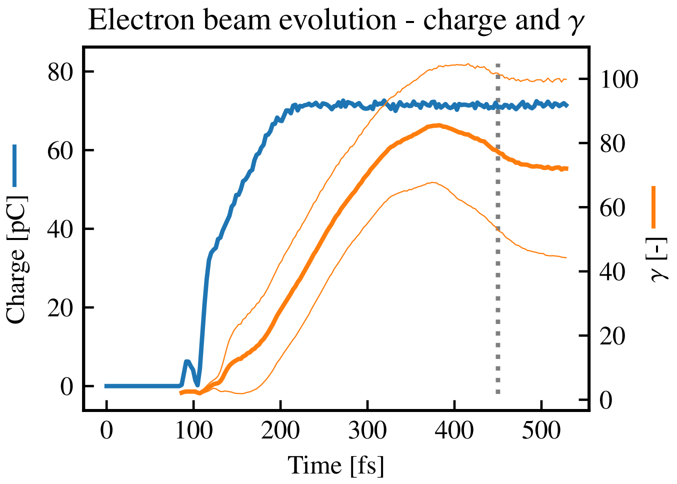


FIG. 6: Circular polarization: temporal evolution of the total beam charge (blue) and the mean energy ($\gamma$, orange), which are similar to the case of linear polarization (figure 2a).

## V. BETATRON RADIATION - DENSITY GRADIENT INJECTION AT $a_0 = 3$

As shown in the main text, for the case of the density gradient the injection is axisymmetric to first approximation. Indeed, asymmetry in the generated betatron radiation is strongly reduced compared to the case of self-injection, to below 10 % (figure 7 (b)). Also, the interplay between the curvature of the electron trajectories and the evolution of $\gamma$ (figure 7 (c) upper panel) is such that emission is not limited to a half-cycle of the betatron oscillation, like in the self-injection case in the main text. Instead, betatron radiation is emitted at comparable power over almost an entire cycle, causing the emission to be nearly symmetric (figure 7 (c) lower panel).

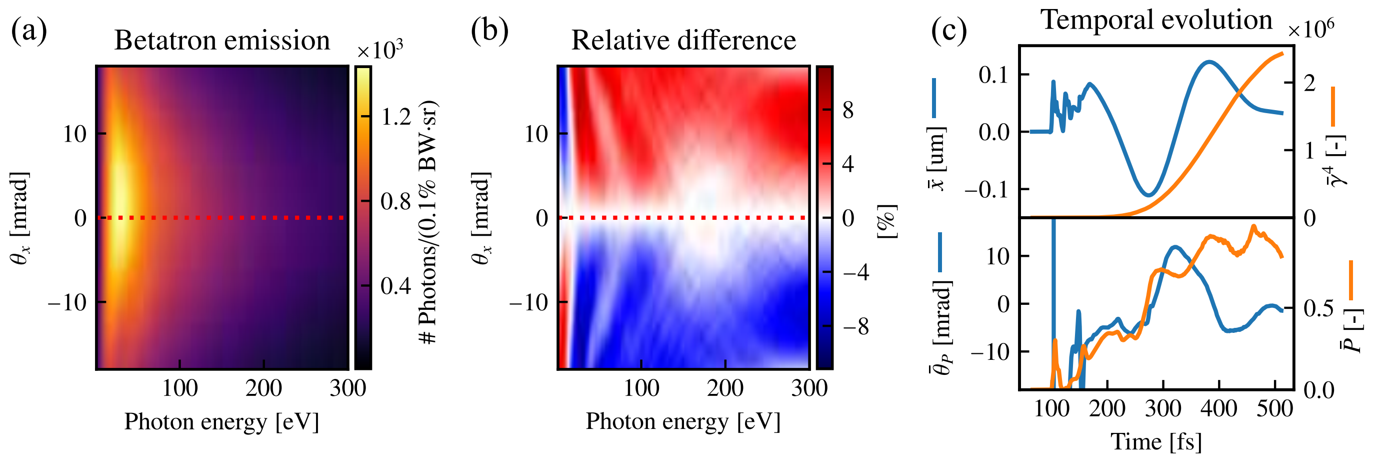


FIG. 7: Asymmetry of the emitted betatron radiation for the density gradient injection case, $a_0 = 3$. (a) Angularly resolved betatron spectrum in for an initial CEP of $\phi_i = 0$. (b) The difference between the spectrum of (a) and the same spectrum for $\phi_i = \pi$, normalized to the sum of the two spectra. The dotted red lines at $\theta_x = 0$ are a guide to the eye. (c) Upper panel: In blue, average transverse coordinate of all electrons that contribute to betatron radiation ($\bar{x}$). In orange, the average value of $\gamma^4$ for these electrons. Lower panel: In blue, the average angle $\bar{\theta}_P$ of the trajectories fo the emitting electrons, weighted by the relative power of the emitters at each timestep. In orange, the power $P$ averaged over all contributing electrons, normalized to its maximum value.

## VI. MOVIES

Movies of the PIC simulations, with the upper panel showing the electron density in shades of green. The laser field and envelope are drawn in red and blue respectively. The lower panel shows the electron beam in phase space.

**Self-injection,** $a_0 = 4, \phi_i = 0$**:**
Note the increasing bubble asymmetry as well as the flattening at the top and bottom of the bubble during propagation.

**Self-injection,** $a_0 = 4, \phi_i = \pi$**:**
Note how this simulation is identical to $\phi_i = 0$, mirrored in the $x = 0$-plane.

**DG-injection,** $a_0 = 3, \phi_i = 0$**:**
Note how the injection is instantanous and seemingly axisymmetric, as opposed to the case of self-injection.

**DG-injection,** $a_0 = 3, \phi_i = \pi$**:**
Note how the injection is instantanous and seemingly axisymmetric, as opposed to the case of self-injection.
